# Supplementary material for: Efficient Pretraining Length Scaling
Source: arXiv:2504.14992 source file (2025-04-24)
Supplement: Supplementary file 1 [file appendix.tex]

\section{Hello World}
%\subsection{Hello World}
